# Supplementary material for: Beat-It: Beat-Synchronized Multi-Condition 3D Dance Generation
Source: arXiv:2407.07554 source file (2024-07-10)
Supplement: Supplementary file 2 [file suppl_ballet.tex]

\begin{table}[h]
    \centering
    \caption{Quantitative results on Jazz Ballet samples of AIST++~\cite{aist++}.}
    \setlength{\tabcolsep}{0.05cm}
    \begin{tabular}{ccccc}
        \toprule
        & \multicolumn{2}{c}{Quality} & \multicolumn{2}{c}{Controllability} \\ \cmidrule(l){2-5}
        \multirow{-2}{*}{Methods} & PFC $\downarrow$     & BAS $\uparrow$     & KPD $\downarrow$         & BAP $\uparrow$        \\ \midrule
        FACT~\cite{aist++}                     & 9.311                & 0.220              & -                        & - \\
        Bailando~\cite{bailando}                 & 4.204                & 0.194              & -                        & - \\ \midrule
        EDGE(keyframes)~\cite{edge}           & 4.571                & \textbf{0.276}     & 1.315                    & - \\
        Ours(beat \& keyframes)                      & \textbf{1.600}       & 0.234              & \textbf{0.407}           & 0.765 \\ \bottomrule
    \end{tabular}
    \label{tab_ballet}
\end{table}
